# Supplementary material for: Path Diffuser: Diffusion Model for Data-Driven Traffic Simulator
Source: arXiv:2509.24995 source file (2025-09-29)
Supplement: Supplementary file 1 [file 6.appendix.tex]

\appendices

  \subsection{Notations}
  \label{sec:notations}

\begin{table}[htbp]
\centering
\caption{Notation}
\label{tab:notation}
\begin{tabular}{ll}
\toprule
\textbf{Symbol} & \textbf{Meaning} \\
\midrule
$x_i, y_i, \theta_i, v_i, c_{i}$ & Initial position, heading, velocity, type of agent i\\
$\vec{x}_i$ & $(x_i, y_i, \theta_i, v_i, c_{i})$ $ \in \sR^5$ \\
$\vec\rvx$ & Initialization of N agents.  $\vec\rvx = \{\vec{x}_i\}_{i=1}^N$\\
$\boldsymbol\tau$ & Trajectory $\boldsymbol\tau \in \sR^{ N\times N_a\times T}$\\
$\boldsymbol\tau_z$ & Latent Trajectory $\boldsymbol\tau \in \sR^{ N\times N_a\times 10}$\\

$N_a, T$ & Attribute dimensions, trajectory duration\\
$N$ & The number of agents\\
$\mathcal{M}$ & Encoded vectorized map\\
\midrule
$\rvx^t$ & Noisy initialization at diffusion step $t$ \\
$\epsilon_\theta$ & Initialization Denoiser \\
$f_\psi$ & Map encoder for agent initializer\\
$M_{a2a}, M_{m2a}$ & Agent-to-agent, map-to-agent attention mask \\
\midrule
$\boldsymbol\tau_z^t$ & Noisy Trajectory Latent diffusion step $t$\\
$\epsilon_\phi$ & Trajectory Denoiser \\
$f_\varphi$ & Map encoder for trajectory generation\\
\midrule
$\bar{\alpha}_t$ & Cumulative product of noise schedule up to $t$ \\
$T_d$ & Maximum diffusion step\\
\midrule
$s_{0}, d_{0}$ & Starting position within a reference lane\\
$(\rvs, \rvd)$ & Candidate trajectory in Frenet space\\
$\boldsymbol\tau_{f}$ & Candidate trajectory in Cartesian space \\
$\mathcal{C}$ & Candidate trajectory in Cartesian Space \\

\bottomrule
\end{tabular}
\end{table}
